# Supplementary material for: Unveiling the Latent Space Geometry of Push-Forward Generative Models
Source: arXiv:2207.10541 source file (2023-05-15)
Supplement: Supplementary file 1 [file unused_old_appendix.tex]

\begin{table}
\centering
\begin{tabular}{l|c|c|c|c|c|c|c}
Dataset & Width  & Acc. & FD & Prec. & Rec. & Dens. & Cov. \\ \hline 
CIFAR-10 %& 16 & 37.0 $\pm$ 0.3 & 1021.9 $\pm$ 18.7  & 46.0 $\pm$ 0.8  & 86.6 $\pm$ 0.4  & 30.5 $\pm$ 0.8  & 54.4 $\pm$ 1.3 \\
& 32 & 53.4 $\pm$ 0.5 & 447.9 $\pm$ 15.6  & 63.8 $\pm$ 0.7  & 82.8 $\pm$ 0.5  & 52.9 $\pm$ 1.3  & 73.0 $\pm$ 1.0\\
& 64 & 60.7 $\pm$ 0.5 & 154.3 $\pm$ 10.8  & 72.1 $\pm$ 0.4  & 81.8 $\pm$ 0.5  & 69.4 $\pm$ 1.5  & 82.9 $\pm$ 0.7 \\
& 128 & 63.4 $\pm$ 0.4  & 94.5 $\pm$ 11.4  & 74.9 $\pm$ 1.0  & 82.2 $\pm$ 0.7  & 74.2 $\pm$ 2.3  & 85.7 $\pm$ 1.0 \\ 
& 256 & 65.0 $\pm$ 0.4 & 75.8 $\pm$ 8.6  & 75.6 $\pm$ 0.4  & 81.9 $\pm$ 0.6  & 76.9 $\pm$ 1.3  & 87.5 $\pm$ 0.8 \\
& 512 & 63.3 $\pm$ 0.6 & 70.8 $\pm$ 6.0 & 76.6 $\pm$ 1.0  & 80.8 $\pm$ 1.0  & 77.5 $\pm$ 2.2  & 87.0 $\pm$ 0.6 \\ \hline
CIFAR-100 %& 16 & \\
& 32 & 20.3 $\pm$ 0.1 &  462.3 $\pm$ 15.1  & 49.3 $\pm$ 0.6  & 82.6 $\pm$ 0.9  & 37.9 $\pm$ 1.6  & 69.5 $\pm$ 1.6 \\
& 64 & 23.7 $\pm$ 0.9 & 286.4 $\pm$ 10.4  & 58.7 $\pm$ 0.7  & 80.6 $\pm$ 0.8  & 49.4 $\pm$ 1.4  & 78.7 $\pm$ 1.6  \\
& 128 & 28.4 $\pm$ 0.3 & 139.1 $\pm$ 11.8 & 65.6 $\pm$ 0.7 & 79.5 $\pm$ 0.6 & 64.3 $\pm$ 2.3 & 85.9 $\pm$ 0.7 \\
& 256 & 32.2 $\pm$ 0.5 & 117.4 $\pm$ 8.2 & 66.0 $\pm$ 0.9 & 79.9 $\pm$ 0.6 & 64.6 $\pm$ 1.8 & 86.4 $\pm$ 0.5  \\
& 512 & 34.4 $\pm$ 0.5 & 115.3 $\pm$ 9.0 & 65.9 $\pm$ 0.5 & 79.8 $\pm$ 0.6 & 64.3 $\pm$ 1.4 & 85.9 $\pm$ 0.5 \\
%Synthetic Mnist & 2 & 34.4 $\pm$ 5.3  & 53.8 $\pm$ 5.8 & 0.5 $\pm$ 0.4 & 59.6 $\pm$ 3.9 & 0.1 $\pm$ 0.1 & 0.2 $\pm$ 0.1\\ 
%& 8 & 72.5 $\pm$ 1.5 & 17.8 $\pm$ 1.4 & 86.2 $\pm$ 1.2 & 57.8 $\pm$ 3.2 & 64.3 $\pm$ 3.1 & 50.6 $\pm$ 1.8  \\
%& 16 & 73.5 $\pm$ 0.8 & 20.4 $\pm$ 1.1 & 88.2 $\pm$ 1.1 & 56.7 $\pm$ 1.8 & 69.5 $\pm$ 1.6 & 49.1 $\pm$ 2.0 \\
%& & \\\hline
\end{tabular}
\caption{Overparametrization study: for a given latent dimension equal to $64$, evolution of GANs' performance when varying the width of the generator. Confidence intervals are computed on 10 checkpoints of the same training. \label{appendix:overparam}}
\end{table}

\section{$G^\star$ illustration}

\begin{tikzpicture}[scale=2]
\coordinate (O) at (0,0) ;
\coordinate (A) at (1,0.58) ;
\coordinate (B) at (-1,0.58) ;
\coordinate (C) at (0,-1.2) ;
\coordinate (F) at (-1,1.1) ;
\coordinate (I) at (0.1,0) ;
\coordinate (J) at (0.1,-1.5) ;
\draw (O) -- (A) ;
\draw (O) -- (B) ;
\draw (O) -- (C) ;
\draw [dashed,color=red] (0.05,0.086) -- (-0.95,0.666) ;
\draw [dashed,color=red] (-0.05,-0.086) -- (-1.05,0.494) ;
\draw [dashed,color=green] (-0.05,0.086) -- (0.95,0.666) ;
\draw [dashed,color=green] (0.05,-0.086) -- (1.05,0.494) ;
%\draw [dashed] (D) -- (F) ;
\draw [dashed,color=blue] (-0.1,0) -- (-0.1,-1.2) ;
\draw [dashed,color=blue] (0.1,0) -- (0.1,-1.2) ;
\draw  [fill=gray!20] (0,0) circle (0.1) ;

\draw (-0.5,-0.5) node[below]{$A_2$} ;
\draw (0.5,-0.5) node[below]{$A_3$} ;
\draw (0.,0.8) node[below]{$A_1$} ;

\draw (1.,-0.15) node[below]{$\partial^\epsilon A_3$};

\draw (-0.2,-1.6) node[below]{Latent space $Z$} ;
\draw (4,-1.6) node[below]{Output space $X$} ;

\coordinate (M1) at (4,0.7) ;
\coordinate (M2) at (3,-1) ;
\coordinate (M3) at (5,-1) ;

\fill[fill=gray!20] (M1)--(M2)--(M3);

\draw (M2) node[below]{$M_2$} ;
\draw (M3) node[below]{$M_3$} ;
\draw (M1) node[above]{$M_1$} ;

\draw [dashed,color=red] (M1) -- (M2) ;
\draw [dashed,color=green] (M1) -- (M3) ;
\draw [dashed,color=blue] (M2) -- (M3) ;

\draw [<-] (0.05,-0.3) -- (0.75,-0.3);
\draw [<-] (0.3,0.1) -- (0.75,-0.3);

\draw [->] (1.25,-0.3) --  (4.4,-0.1);
\draw [->] (1.25,-0.3) --  (4.0,-0.95);

\draw (M1) [fill=black] circle (0.03) ;
\draw (M2) [fill=black] circle (0.03) ;
\draw (M3) [fill=black] circle (0.03) ;
\end{tikzpicture}

\begin{table}
\begin{tabular}{l|c|c|c|c|c|c|c}
Dataset & L. Dim.  & Acc. & FD & Prec. & Rec. & Dens. & Cov. \\ \hline 
Mnist & 2 & 44.3 $\pm$ 2.5 & 112.3 $\pm$ 22.6 & 2.9 $\pm$ 1.0 & 89.1 $\pm$ 2.0 & 0.9 $\pm$ 0.3 & 2.1 $\pm$ 0.5 \\ 
& 4 & 59.4 $\pm$ 0.7 & 36.4 $\pm$ 9.3 & 75.7 $\pm$ 1.8 & 91.5 $\pm$ 0.5 & 47.9 $\pm$ 2.2 & 66.0 $\pm$ 2.0 \\
& 6 & 83.9 $\pm$ 0.4 & 15.4 $\pm$ 3.0 & 90.0 $\pm$ 0.7 & 92.4 $\pm$ 0.7 & 76.3 $\pm$ 2.0 & 85.8 $\pm$ 0.4 \\
 & 8 & 84.7 $\pm$ 0.4 & 18.2 $\pm$ 3.4 & 91.1 $\pm$ 0.7 & 92.3 $\pm$ 0.5 & 81.3 $\pm$ 2.2 & 87.1 $\pm$ 0.8 \\ 
  & 10 & 86.7 $\pm$ 0.4 & 10.7 $\pm$ 2.6 & 93.3 $\pm$ 0.5 & 91.5 $\pm$ 0.5 & 89.0 $\pm$ 2.2 & 89.8 $\pm$ 0.7 \\
  & 12 & 87.4 $\pm$ 0.4 & 7.2 $\pm$ 1.6 & 94.6 $\pm$ 0.5 & 91.5 $\pm$ 0.5 & 94.3 $\pm$ 2.0 & 91.8 $\pm$ 0.7 \\
  & 16 & 86.9 $\pm$ 0.4 & 11.0 $\pm$ 1.0 & 93.8 $\pm$ 0.3 & 91.8 $\pm$ 0.6 & 92.2 $\pm$ 0.9 & 90.7 $\pm$ 0.5 \\
  & 32 & 90.3 $\pm$ 0.4 & 10.4 $\pm$ 1.6 & 93.6 $\pm$ 0.3 & 91.6 $\pm$ 0.7 & 91.8 $\pm$ 1.7 & 90.3 $\pm$ 0.6 \\
  & 64 & 90.4 $\pm$ 0.3 & 13.3 $\pm$ 2.6 & 93.2 $\pm$ 0.4 & 92.3 $\pm$ 0.5 & 90.1 $\pm$ 2.0 & 90.2 $\pm$ 0.8 \\
  & 128 & 87.0 $\pm$ 0.4 &  11.0 $\pm$ 2.3 & 93.6 $\pm$ 0.3 & 91.8 $\pm$ 0.4 & 91.6 $\pm$ 1.5 & 90.4 $\pm$ 0.7 \\ \hline 
CIFAR-10 & 2 & 19.1 $\pm$ 1.1 & 408.3 $\pm$ 23.3 & 6.4 $\pm$ 0.9 & 79.5 $\pm$ 1.3 & 1.8 $\pm$ 0.3 & 3.9 $\pm$ 0.4 \\
& 4 & 27.4 $\pm$ 1.0 & 298.6 $\pm$ 38.1 & 59.2 $\pm$ 0.8 & 78.9 $\pm$ 0.8 & 42.9 $\pm$ 0.6 & 65.9 $\pm$ 0.7 \\
& 6 & 42.7 $\pm$ 0.6 & 142.6 $\pm$ 5.4 & 69.4 $\pm$ 0.6 & 76.6 $\pm$ 0.5 & 60.3 $\pm$ 1.1 & 76.3 $\pm$ 0.8\\
& 8 & 44.6 $\pm$ 0.6 & 174.7 $\pm$ 9.6 & 69.7 $\pm$ 0.7 & 79.6 $\pm$ 0.5 & 61.0 $\pm$ 1.4 & 77.8 $\pm$ 1.0\\
& 10 & 53.7 $\pm$ 0.4 & 134.7 $\pm$ 7.4 & 72.7 $\pm$ 0.6 & 76.6 $\pm$ 0.6 & 67.6 $\pm$ 1.3 & 80.4 $\pm$ 1.0 \\
& 12 & 58.2 $\pm$ 0.3 & 131.8 $\pm$ 8.5 & 74.0 $\pm$ 0.5 & 76.1 $\pm$ 0.6 & 71.3 $\pm$ 1.6 & 82.0 $\pm$ 1.1\\
& 14 & 60.1 $\pm$ 0.4 & 115.5 $\pm$ 12.7 & 74.0 $\pm$ 0.5 & 77.7 $\pm$ 0.8 & 72.4 $\pm$ 1.4 & 82.8 $\pm$ 0.9 \\
& 16 & 60.7 $\pm$ 0.4 & 145.9 $\pm$ 8.9 & 73.2 $\pm$ 0.7 & 78.5 $\pm$ 0.7 & 66.9 $\pm$ 1.3 & 79.6 $\pm$ 0.7\\
& 32 & 63.5 $\pm$ 0.2 & 126.5 $\pm$ 5.9 & 74.5 $\pm$ 0.5 & 79.1 $\pm$ 0.4 & 70.9 $\pm$ 1.5  & 82.0 $\pm$ 0.9 \\
& 64 & 64.0 $\pm$ 0.3 & 124.6 $\pm$ 4.5 & 74.0 $\pm$ 0.6 & 79.2 $\pm$ 0.3 & 71.2 $\pm$ 1.8 & 82.7 $\pm$ 1.0 \\ 
& 128 & 63.6 $\pm$ 0.4 & 132.6 $\pm$ 7.8 & 73.8 $\pm$ 0.5 & 79.2 $\pm$ 0.6 & 69.7 $\pm$ 1.2 & 82.1 $\pm$ 0.6 \\ \hline
 CIFAR-100 & 2 & 10.7 $\pm$ 1.4 & 2826.7 $\pm$ 837.3 & 1.4 $\pm$ 0.2 & 70.2 $\pm$ 1.1 & 0.3 $\pm$ 0.1 & 0.7 $\pm$ 0.1 \\ 
 & 8 & 15.2 $\pm$ 0.2 & 1112.3 $\pm$ 56.9 & 59.5 $\pm$ 0.8 & 62.8 $\pm$ 0.6 & 49.8 $\pm$ 1.6 & 70.5 $\pm$ 1.1\\
& 16 & 21.8 $\pm$ 0.3 & 1270.9 $\pm$ 89.7& 63.6 $\pm$ 1.3 & 61.3 $\pm$ 0.8 & 57.2 $\pm$ 2.8 & 73.9 $\pm$ 1.2 \\
& 32 & 23.9 $\pm$ 0.4 & 1068.0 $\pm$ 91.5 & 65.3 $\pm$ 0.4 & 62.1 $\pm$ 0.6 & 60.6 $\pm$ 1.1 & 77.4 $\pm$ 0.6 \\ 
& 64 & 25.1 $\pm$ 0.4 & 822.2 $\pm$ 50.5 & 66.5 $\pm$ 0.6 & 61.5 $\pm$ 0.8 & 64.0 $\pm$ 1.4 & 78.5 $\pm$ 0.8 \\
& 128 & 23.5 $\pm$ 0.3 & 963.0 $\pm$ 74.2 & 65.2 $\pm$ 0.7 & 62.2 $\pm$ 1.0 & 61.7 $\pm$ 1.6 & 77.4 $\pm$ 0.8 \\ 
& 256 & 21.2 $\pm$ 0.3 & 1086.6 $\pm$ 78.0 & 66.0 $\pm$ 0.5 & 60.2 $\pm$ 0.8 & 63.9 $\pm$ 1.2 & 78.1 $\pm$ 0.7 \\ 
& 512 & 20.6 $\pm$ 0.4 & 1128.7 $\pm$ 95.3 & 66.8 $\pm$ 0.6 & 61.1 $\pm$ 0.6 & 63.0 $\pm$ 1.2 & 77.6 $\pm$ 0.8 \\ \hline
CIFAR-3 & 2 & 44.8 $\pm$ 2.0 & 473.9 $\pm$ 55.0 & 5.3 $\pm$ 0.5 & 69.9 $\pm$ 2.1 & 1.5 $\pm$ 0.2 & 2.7 $\pm$ 0.4 \\
& 6 & 72.4 $\pm$ 0.4 & 169.2 $\pm$ 13.1 & 73.4 $\pm$ 0.8 & 69.7 $\pm$ 1.5 & 65.6 $\pm$ 1.5 & 72.7 $\pm$ 1.3 \\
& 8 & 78.4 $\pm$ 0.5 & 144.6 $\pm$ 8.2 & 74.9 $\pm$ 0.5 & 72.5 $\pm$ 1.4 & 71.0 $\pm$ 1.6 & 75.8 $\pm$ 1.7 \\ 
& 12 & 80.6 $\pm$ 0.4 & 135.2 $\pm$ 6.4 & 77.5 $\pm$ 0.5 & 71.2 $\pm$ 1.3 & 76.5 $\pm$ 1.1 & 78.3 $\pm$ 1.7 \\
& 16 & 80.9 $\pm$ 0.3 & 113.3 $\pm$ 9.0 & 78.7 $\pm$ 0.5 & 71.8 $\pm$ 1.5 & 80.7 $\pm$ 1.4 & 80.4 $\pm$ 1.4 \\ 
& 128 & 80.6 $\pm$ 0.1 & 115.3 $\pm$ 8.4 & 80.5 $\pm$ 0.7 & 70.4 $\pm$ 1.7 & 87.1 $\pm$ 2.1 & 82.7 $\pm$ 1.3 \\ \hline
Synthetic CIFAR-10 & 2 & 22.8 $\pm$ 2.2 & 234.6 $\pm$ 12.1 & 7.3 $\pm$ 1.3 & 71.7 $\pm$ 1.1 & 2.2 $\pm$ 0.4 & 4.6 $\pm$ 0.8 \\
& 4 & 33.8 $\pm$ 0.8 & 143.2 $\pm$ 15.0 & 60.3 $\pm$ 0.8 & 72.5 $\pm$ 0.8 & 44.4 $\pm$ 1.3 & 68.9 $\pm$ 1.2 \\ 
& 8 & 47.0 $\pm$ 0.6 & 85.5 $\pm$ 4.7 & 70.2 $\pm$ 0.3 & 72.5 $\pm$ 0.9 & 64.6 $\pm$ 0.6 & 83.2 $\pm$ 0.6 \\ 
& 10 & 52.6 $\pm$ 0.3 & 87.6 $\pm$ 5.4 & 70.4 $\pm$ 0.6 & 73.1 $\pm$ 0.7 & 66.2 $\pm$ 1.8 & 84.3 $\pm$ 0.7 \\
& 12 & 55.3 $\pm$ 0.4 & 84.3 $\pm$ 4.9 & 70.0 $\pm$ 0.5 & 73.5 $\pm$ 0.6 & 64.8 $\pm$ 1.2 & 83.6 $\pm$ 0.6 \\ 
& 16 & 59.1 $\pm$ 0.4 & 76.4 $\pm$ 6.1 & 71.6 $\pm$ 0.6 & 72.9 $\pm$ 1.2 & 68.7 $\pm$ 1.8 & 85.1 $\pm$ 0.4 \\
& 32 & 52.8 $\pm$ 0.2 & 73.4 $\pm$ 6.3 & 72.6 $\pm$ 0.5 & 72.2 $\pm$ 0.7 & 69.5 $\pm$ 1.4 & 85.7 $\pm$ 0.5 \\ 
& 128 &  58.7 $\pm$ 0.3 & 88.3 $\pm$ 6.2 & 70.1 $\pm$ 0.6 & 73.3 $\pm$ 0.6 & 66.3 $\pm$ 1.4 & 84.2 $\pm$ 0.8 \\ 

 \\ \hline 
Synthetic Mnist & 2 & 34.4 $\pm$ 5.3  & 53.8 $\pm$ 5.8 & 0.5 $\pm$ 0.4 & 59.6 $\pm$ 3.9 & 0.1 $\pm$ 0.1 & 0.2 $\pm$ 0.1\\ 
& 8 & 72.5 $\pm$ 1.5 & 17.8 $\pm$ 1.4 & 86.2 $\pm$ 1.2 & 57.8 $\pm$ 3.2 & 64.3 $\pm$ 3.1 & 50.6 $\pm$ 1.8  \\
& 16 & 73.5 $\pm$ 0.8 & 20.4 $\pm$ 1.1 & 88.2 $\pm$ 1.1 & 56.7 $\pm$ 1.8 & 69.5 $\pm$ 1.6 & 49.1 $\pm$ 2.0 \\
& & \\\hline
\end{tabular}
\caption{Performance of GANs when varying latent space dimension. Confidence intervals are computed on 10 checkpoints of the same training. }
\end{table}

\begin{figure}[H]
    \subfloat[$n=3$.]
    {   
        \includegraphics[width=0.40\linewidth]{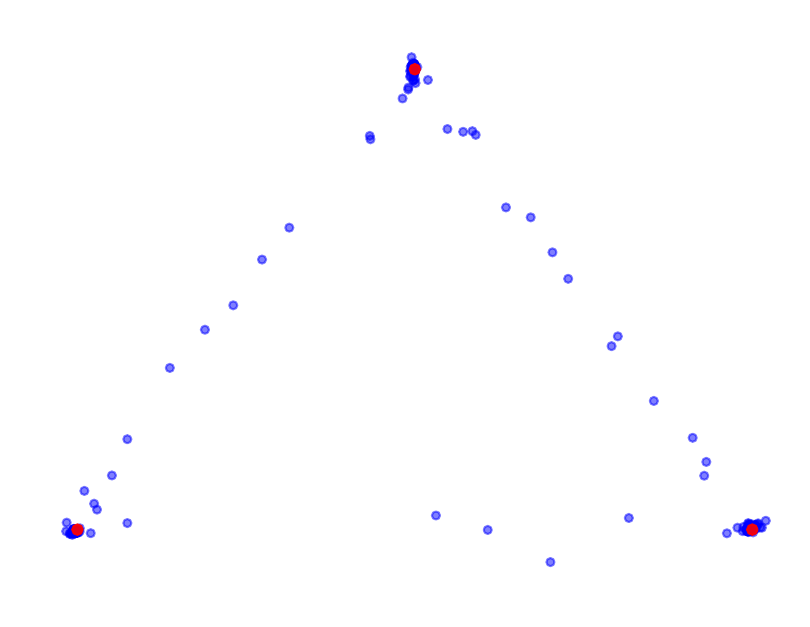}
    }
    \subfloat[]
    {   
        \includegraphics[width=0.40\linewidth]{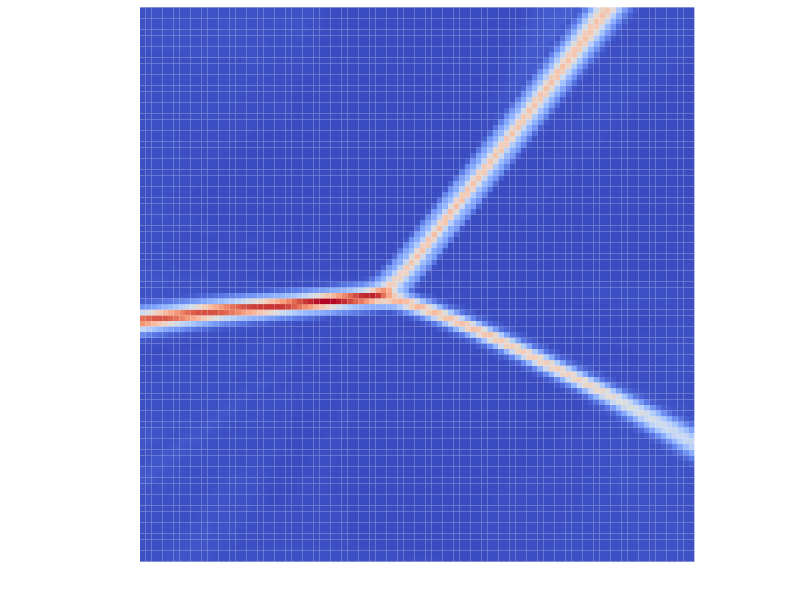}
    }
    \subfloat[$n=5$.]
    {   
        \includegraphics[width=0.40\linewidth]{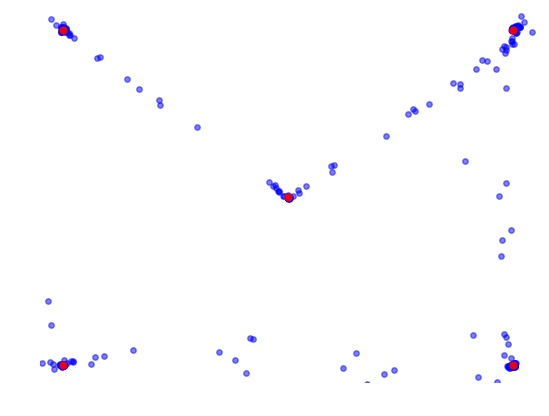}
    }
    \subfloat[]
    {   
        \includegraphics[width=0.40\linewidth]{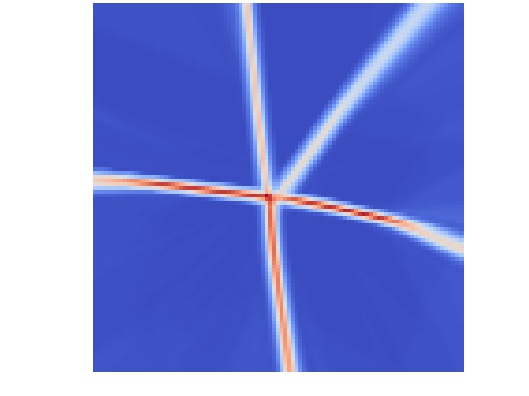}
    }
    \subfloat[$n=6$.]
    {   
        \includegraphics[width=0.40\linewidth]{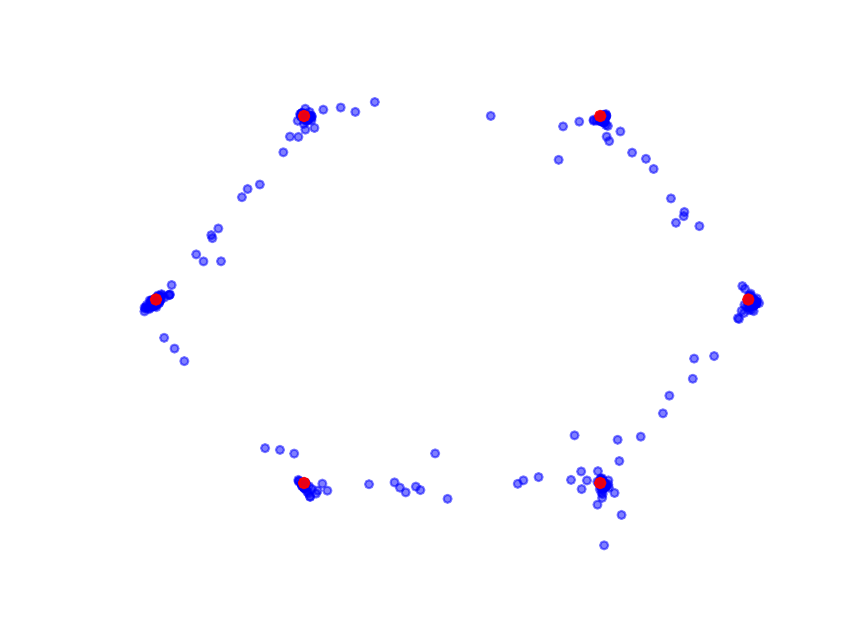}
    }
    \subfloat[]
    {   
        \includegraphics[width=0.40\linewidth]{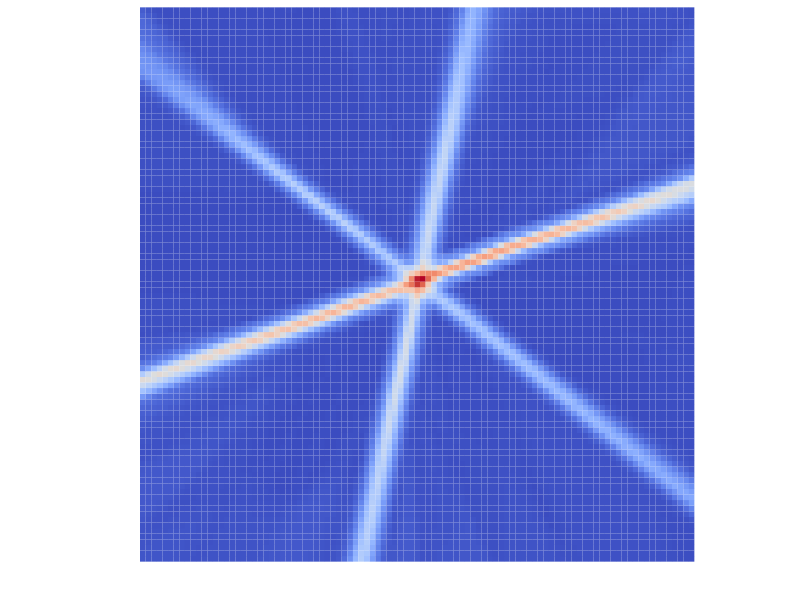}
    }
    \caption{\label{fig:MST_synthetic1} Illustration of WGANs on few-shot learning ($n=8, 16, 32$).\label{fig:1}}
\end{figure}

\section{Technical results}
\subsection{Proof of Theorem \ref{th:th1}}

\begin{lemma}[From \citet{tanielian2020learning}, Lemma 3]
    Let $\mu$ be a probability distribution associated with a uniformly continuous probability density function $f_\mu$. Assume that there exists constants $a_1>0, a_2>0$ such that for all $x \in E$, we have $a_1 < f_\mu(x) \leqslant a_2$. Then,  
    \begin{align*}
        R_{\text{min}} \underset{n \to \infty}{\longrightarrow} 0 \ \text{a.s.} \quad \text{and} \quad R_{\text{min}}^d \underset{n \to \infty}{\longrightarrow} \infty \ \text{a.s.} \\
        R_{\text{max}} \underset{n \to \infty}{\longrightarrow} 0 \ \text{a.s.} \quad \text{and} \quad R_{\text{max}}^d \underset{n \to \infty}{\longrightarrow} \infty \ \text{a.s.}         
    \end{align*}
\end{lemma}

\begin{lemma}[Coverage]
    Let $\mu$ be a probability distribution associated with a uniformly continuous probability density functions $f_\mu$ such that there exists constants $a_1>0, a_2>0$ such that for all $x \in E$, we have $a_1 < f_\mu(x) \leqslant a_2 $. Let $\nu$ be a singular probability distribution. Also, let $D_\mu, D_\nu$ be datasets sampled from $\nu^n, \mu^n$. If $\mu$ is an estimator for $\nu$, then
    \begin{align*}
        \text{a) for all } x \in D_\mu,& \ \mathds{1}_{ 
        \{\exists y \in D_\nu, y \in B_k(x)\}} \underset{k \to \infty}{\rightarrow} \mathds{1}_{\emph{supp}(\nu)}(x) \quad \text{in proba.} \\
        \text{b) for all } y \in D_\nu,& \ \sum_{x \in D_\mu} \ \mathds{1}_{\{y \in B_k(x)\}} \underset{k \to \infty}{\rightarrow} \mathds{1}_{\emph{supp}(\mu)}(x) \quad \text{in proba.},
    \end{align*}
\end{lemma}
where $B_k(X)$ refers to the set of k Nearest Neighbor of the point $X$ with respect to the Euclidean distance.

So we know that $B_k(X_i) \underset{k \to \infty}{\to} 0 \ \text{a.s.}$. Assume that $X_i \in S_{G \sharp \gamma}$, it is clear that $\mathds{1}_{\{\exists j \in [1,M], Y_j \in B_k(X_i)\}} \underset{k \to \infty}{\to} 0 \ \text{a.s.}$. Now, assume that $X_i \in S_{G \sharp \gamma}$. 

\begin{proof}
    Thus, we want to show that 
    \begin{equation*}
        \text{  for all } x \in D_\mu, \ \alpha_{\varphi(n)}^n(x) \underset{n \to \infty}{\rightarrow} \mathds{1}_{\emph{supp}(\nu)}(x) \quad \text{a. s.}
    \end{equation*}
    
    First, let's assume that $x \notin S_\nu$. \citet[][Lemma  2.2]{biau2015lectures} have shown that 
    \begin{equation*}
        \underset{n \to \infty}{\lim} \|x_{(\varphi(n))}-x\| = \inf \{\|x-y\| \mid y \in S_\nu \} \quad \text{a.s.}
    \end{equation*}
    As $S_\nu$ is a closed set - e.g. \cite{kallenberg2006foundations} - we have 
    \begin{equation*}
        \underset{n \to \infty}{\lim} \ \|x-x_{(\varphi(n))}\| > 0 \quad \text{a.s.}
    \end{equation*}
    and 
    \begin{equation*}
        \text{for all } y \in D_\nu, \underset{{n} \to \infty}{\lim} \ \|y-y_{({\varphi(n)})}\| = 0 \quad \text{a.s.}
    \end{equation*}
    Thus, $\underset{n \to \infty}{\lim} \alpha_{\varphi(n)}^n(x) = 0 \quad \text{a.s.}$.    
    
    Now, let's assume that $x \in S_\nu$. We want $\exists y \in S_\nu$ such that $\|x-y\| \leqslant \|x-x_{(k)}\|$. Noting $y_{(1)}$ the nearest neighbor within $D_\nu$ from $x$ w.r.t. the Euclidean distance, this is equivalent to $\|x-y_{(1)}\| \leqslant \|x-x_{(k)}\|$.
    
    Using \citet[][Theorem 4.2]{biau2015lectures}, we have that:
    \begin{equation*}
        \frac{k}{nV_d \|x-x_{(k)}\|^d } \to f_\nu(x),
    \end{equation*}
    where $f_\nu$ denotes the density function and $V_d$ the volume of the unit sphere in $\mathds{R}^d$. Thus, 
    \begin{equation*}
        \|x-x_{(k)}\| = O\Big( \big(\frac{k}{n}\big)^{1/d} \Big).
    \end{equation*}
    Using \citet[][Theorem 2.2]{biau2015lectures}, we have that:
    \begin{equation*}
        \|x-y_{(1)}\| = o(n^{1/d}).
    \end{equation*}
    Thus, we conclude.
    %(Strong uniform consistency) with Theorem 2.2: if X is singular: goood! Thus, it is now clear that, $\mu(S_\nu \Delta S_\nu^n) \to 0$ in probability. Finally, given $x \in S_\mu$, we have $\mu(x \in S_\nu^n) = \nu(\alpha_{\varphi(n)}^n(x) = 1) \to 1 $ in probability.
    %We have $\mathds{1}_{\{\exists y \in D_\nu, y \in B_k(x)\}}$:
    %We have $\|x-x_{(k)}\| $. 
    % \begin{equation*}
    %     R_{\text{min}}^\mu = \underset{x \in D_\mu}{\min} \|x-x_{(k)}\| \leqslant \|x-x_{(k)}\| \leqslant   R_{\text{max}}^\nu = \underset{x \in D_\mu}{\max} \|x-x_{(k)}\| \underset{k \to 0}{\longrightarrow} 0 \quad \text{in proba.}.
    % \end{equation*}
    % It is clear that :
    % \begin{equation}\label{eq:bounding_s_mu_n}
    %      \bigcup_{y \in D_\nu} B(y, R_{\text{min}}) \subseteq S_\nu^n \subseteq \bigcup_{y \in D_\nu} B(y, R_{\text{max}}),
    % \end{equation}
    % where $S_\nu^n = \bigcup_{y \in D_\nu} B(y, \|y-y_{(\varphi(n))}\|))$. 
    % Besides, combining Lemma \ref{lem:auxiliary_lemma} with \citet[][Theorem 1]{devroye1980detection}, we have that:
    % \begin{align*}
    %     \nu(S_\nu \Delta \bigcup_{y \in D_\nu} B(y, R_{\text{min}})) \underset{n \to 0}{\longrightarrow} 0 \quad \text{in proba.} \\
    %     \nu(S_\nu \Delta \bigcup_{y \in D_\nu} B(y, R_{\text{max}})) \underset{n \to 0}{\longrightarrow} 0 \quad \text{in proba.} \\
    % \end{align*}
    % where $\Delta$ here refers to the symmetric difference.
\end{proof}

\section{Gaussian inequalities}
 \begin{theorem}
     Let us denote $\Omega$ a m-simplicial cluster with gaussian measure $\nu$. Let us denote A a partition with same gaussian measure $\nu$ than $\Omega$. Then, we have, for every $\epsilon > 0$,
 \begin{equation}
     \gamma \big((\partial A)^\epsilon \big) \geqslant \gamma \big((\partial \Omega)^\epsilon \big)
 \end{equation}
 \end{theorem}

\subsection{Computation/Lower-bounding of the boundaries}
We can now develop a lower-bound measure for $\gamma^{d} \big((\partial \Omega)^\epsilon \big)$:
\begin{equation}
    \gamma \big((\partial \Omega)^\epsilon \big) = \sum_{i=1}^m \gamma \big((\partial \Omega_{i})^{\epsilon} \big)
\end{equation}
\begin{equation}
     \gamma \big((\partial \Omega_{i})^{\epsilon} \big) = \sum_{j=1,j\neq i}^m \gamma \big((\partial \Omega_{i,j})^{\epsilon} \big) - \gamma \big((\partial \Omega_{i,j})^{\epsilon} \cap (\cup_{k<j}\partial \Omega_{i,k})^{\epsilon} \big) 
\end{equation}

Moreover, for a given interface $\partial \Omega_{i,j}^{\epsilon}$, we can approximate (slightly underestimate) the measure of the $\epsilon$-enlargement :
\begin{equation}
    \gamma(\partial \Omega_{i,j}^{\epsilon}) = \gamma^{d-1}(\partial \Omega_{i,j}) \times \Big(\Phi(\epsilon) - 1/2 \Big)
\end{equation}

Geometry of $\partial \Omega_{i,j}$: it is a convex cone contained in an hyperplane formed by $m-2$ vectors. where each pair of vector has angle $\cos^{-1}(\frac{1}{m-1})$ (comes from the generalization of a tetrahedron in $d=m-1$ dimensions).

%\subsubsection{Bound from \cite{schechtman2012approximate}}In \cite{schechtman2012approximate}, the authors develop the following bound on the gaussian measure of the $\epsilon$-enlargement of the boundaries, in the equal-volume case and for $m \leqslant d$:
% \begin{align*}
%     c \epsilon \sqrt{\log(m)} &\leqslant \gamma(\partial \Omega^\epsilon) \leqslant C \epsilon \sqrt{\log(m)} \\
%     c \epsilon \sqrt{\log(m)} &\leqslant 1 - \alpha \leqslant C \epsilon \sqrt{\log(m)}
% \end{align*}

%\subsubsection{Discussion on dimension/number of modes}If $m \leqslant d$ (less or equal clusters than dimension), it is clear that free dimensions appear: one can construct a simplicial cluster by setting a cluster's representant $x_i$ to 0 everywhere and 1 on dimension $i$. In this setting, there is a $(d-m+2)$-dimensional space which is a common boundary to all clusters (see, for example, the "propeller" shape for $d=3$ and $m=3$ \cite{heilman2013solution}). Since the gaussian measure is rotation invariant and a product measure, one can thus integrate out these free dimensions, and study the problem in $\mathds{R}^{m-1}$.

\section{Theoretical results}
\subsection{Result on Wasserstein distance}
\begin{theorem}
    Let assume that latent variable $\gamma$ is the uniform distribution. We have that:
    \begin{equation*}
        W(\mu_n, G_A^\star \sharp \gamma) \leqslant \underset{G \in \mathscr{G}_\mathscr{A}}{\inf} \ W(\mu_n, G \sharp \gamma)
    \end{equation*}
\end{theorem}

\begin{proof}
Let $\mu \in \mu(A)$ and $T_\mu$ be the optimal transport between $\mu$ and $\mu_n$. Let $G$ be the generator associated with $\mu$.
\begin{align*}
    W(\mu_n, \mu) &= \int_{\mathds{R}^D} \|G(z)-T_\mu(G(z))\| \rm\gamma (dz) = \sum_{i=1}^n \int_{A_i} \|G(z)-X_i\| \rm\gamma (dz) \\
    &= \sum_{i=1}^n \int_{A_i^{-\varepsilon_i}} \|G(z)-X_i\| \rm\gamma (dz) + \sum_{i=1}^n \int_{A_i \backslash A_i^{-\varepsilon_i}} \|G(z)-X_i\| \rm\gamma (dz) \\
    & \geqslant \sum_{i=1}^n \int_{A_i \backslash A_i^{-\varepsilon_i}} \|G(z)-X_i\| \rm\gamma (dz)\\
    & \geqslant \sum_{i=1}^n \int_{A \backslash A_i^{-\varepsilon_i}} \|G_A^\star(z)-X_i\| \rm\gamma (dz) \\
    & \text{(otherwise contradiction with $L$-Lipschitzness of $G$)} \\
    &\geqslant W(\mu_n, \mu_A^\star).
\end{align*}

\textbf{Assume $n=2$:} \\ For any $z \in A_{1,2}$, we define $(z_1   z_2) \in A_1^{-\varepsilon_1}, A_2^{-\varepsilon_2}$ such that:
\begin{equation*}
    z_1 = \underset{z' \in A_1^{-\varepsilon_1}}{\min} \ \|z-z'\| \quad \text{and} \quad z_2 = \underset{z' \in A_2^{-\varepsilon_2}}{\min} \ \|z-z'\|
\end{equation*}

\begin{assumption}
    We assume that for any continuous function:
    \begin{equation*}
        \sum_{i=1}^2 \int_{A_i \backslash A_i^{-\varepsilon_i}} f(z) \rm\gamma (dz) = \int_{A_{1,2}} \big(\int_{z=z_1}^{z_2} f(u) \rm \rm \gamma(du) \big) dz
    \end{equation*}
\end{assumption}

Let a tuple $(z_1, z, z_2)$ defined as above. We have that:
\begin{align*}
    &\int_{z_1}^{z_2} \|G(z)-T_\mu(G(z))\| \rm\gamma (dz) - \int_{z_1}^{z_2} \|G_A^\star(z)-T_\mu(G(z))\| \rm\gamma (dz) \\
    &= \int_{z_1}^{z} \|G(z)-T_\mu(G(z))\| - \|G_A^\star(z)-T_\mu(G(z))\| \rm\gamma (dz) + \int_{z}^{z_2} \|G(z)-T_\mu(G(z))\|-\|G_A^\star(z)-T_\mu(G(z))\| \rm\gamma (dz) \\
    &=\int_{z_1}^{z} \|G(z)-X_1\|-\|G_A^\star(z)-X_1\| \rm\gamma (dz) + \int_{z}^{z_2} \|G(z)-X_2\|-\|G_A^\star(z)-X_2\| \rm\gamma (dz)
\end{align*}
Let $f$ the function defined on $[z_1, z]$ be such that:
\begin{equation*}
    f(z) = \|G_A^\star(z)-X_1\|-\|G(z)-X_1\|.
\end{equation*}
It is clear that the function $f$ is increasing (otherwise it contradicts the $L$-Lipschitzness of $G$). Consequently, for all $z \in [z_1, z]$, we have $0 \leqslant f(z) \leqslant f(z)$. 
Conversely, for all $z \in [z, z_2]$, we have that
\begin{equation*}
    g(z) = \|G_A^\star(z)-X_2\|-\|G(z)-X_2\|,
\end{equation*}
is a decreasing function with for all $z \in [z, z_2]$, $g(z) \leqslant g(z) = f(z)$ since on the boundary we have that $\|x-X_1\|-\|x-X_2\| = w_i-w_j$.

Therefore we have that:
\begin{align*}
    &\int_{z_1}^{z_2} \|G(z)-T_\mu(G(z))\| \rm\gamma (dz) - \int_{z_1}^{z_2} \|G_A^\star(z)-T_\mu(G(z))\| \rm\gamma (dz) \\
    &=\int_{z_1}^{z} -f(z) \rm\gamma (dz) + \int_{z}^{z_2} -g(z)\rm\gamma (dz) \\
    & \geqslant \int_{z_1}^{z} -f(z) \rm\gamma (dz) + \int_{z}^{z_2} -g(z)\rm\gamma (dz) \\
    & \text{(since $-f$ is decreasing and $-g$ increasing)}\\
    &\geqslant 0.
\end{align*}
\end{proof}

\subsection{Proof of Theorem \ref{th:optimal_precision_GANs}}
\begin{proof}
    By definition from $G^\star$, we have that its equilibrium is equal to $1$ since $\gamma(A_1) = \hdots = \gamma(A_m)$. 
    
    Then, let $i \in [1, n]$ since $L \geqslant d \sqrt{m}$, there exists $x_i \in A_i$ and $\eta \geqslant 0$ such that $\mathds{B}(x_i, \eta) \subset \big(A_i \setminus \bigcup_{j \neq i} A_i^\varepsilon \big)$. Thus, for all $z \in \mathds{B}(x_i, \eta)$, we have $G^\star(z) = X_i$. Thus, $\text{coverage}=1$.
    
    Now, let's show that $G^\star \in \mathcal{G}_L$. To begin with, we have $\mathds{R}^d = \partial^\varepsilon \mathcal{A} \bigcup \big(\mathds{R}^d \setminus \partial^\varepsilon \mathcal{A} \big)$. 
    
    \begin{equation*}
        \mathds{R}^d \setminus \partial^\varepsilon \mathcal{A} = \bigcup_{i=1}^n A_i \textbackslash \big( (\cup_{j \neq i} A_j)^\varepsilon \cap A_i \big), 
    \end{equation*}
    and, we know that for each $i \in [1,n]$, $G^\star(z)$ is constant and thus $L$-Lipschitz.
    
    Now,
    \begin{equation*}
        \partial^\varepsilon \mathcal{A} = \bigcup_{i=1}^n \big( \cup_{j \neq i} A_j\big)^\varepsilon \textbackslash \big(\cup_{j \neq i} A_j \big) = \bigcup_{\substack{S \in \mathcal{P}([1,n]) \\ \text{card}(S) \geqslant 2}} \ \bigcap_{i \in S} A_i^\varepsilon.
    \end{equation*}
    Now, let $S \in \mathcal{P}([1,n])$ with $\text{card}(S)=k\geqslant2$. Let $z, z' \in S^2$. Let $\alpha = (\alpha_1,\hdots, \alpha_k)$ and $\beta = (\beta_1, \hdots, \beta_k)$ be two vectors, both in $\mathds{R}^k$, such that for all $i \in [1, k]$:
    \begin{equation*}
        \alpha_i = \frac{d(z, (A_i^{\varepsilon})^\complement)}{\sum_{j \in \mathcal{A}_z} d(z, (A_j^{\varepsilon})^\complement)} \quad \text{and} \quad \beta_i = \frac{d(z', (A_i^{\varepsilon})^\complement)}{\sum_{j \in \mathcal{A}_z} d(z', (A_j^{\varepsilon})^\complement)} 
    \end{equation*}
    
    We have that 
    \begin{align*}
        \|G(z) - G(z')\| &= \| (1-\sum_{i \neq 1} \alpha_i) X_1 - (1-\sum_{i \neq 1} \beta_i) X_1 + \sum_{i \neq 1} \alpha_i X_i - \sum_{i \neq 1} \beta_i X_i \| \\
        &= \| \sum_{i \neq 1} (\alpha_i - \beta_i) (X_1 - X_i) \| \\
        & \leqslant \underset{(i,j) \in [1,n]^2}{\max} \|X_i - X_j\|  \ \|\alpha - \beta \|, \\
        & \leqslant \underset{(i,j) \in [1,n]^2}{\max} \|X_i - X_j\|  \ \|h(z) - h(z') \|,
    \end{align*}
    where $h$ is the function from $\mathds{R}^d \to \mathds{R}^k$ be defined as:
    \begin{equation*}
        h(z) = (\frac{d(z, (A_1^{\varepsilon})^\complement)}{\sum_{i \in \mathcal{A}_z} d(z, (A_i^{\varepsilon})^\complement)}, \hdots, \frac{d(z, (A_k^{\varepsilon})^\complement)}{\sum_{i \in \mathcal{A}_z} d(z, (A_i^{\varepsilon})^\complement)}).
    \end{equation*}
    
    We can write $h = f \circ g$ with $f$ the function defined from $\mathds{R}^d \to \mathds{R}^k$ by
    \begin{equation*}
        f(z) = \Big(d(z, (A_1^{\varepsilon})^\complement), \hdots, d(z, (A_k^{\varepsilon})^\complement) \Big),
    \end{equation*}
    and $g$ the function defined on $\mathds{R}^k \setminus \{0\}$ by 
    \begin{equation*}
        g(z) = \frac{z}{\|z\|_1}
    \end{equation*}
    
    We have that $f$ is a $\sqrt{k}$-Lipschitz functions (given that $z \mapsto d(z, (A_k^{\varepsilon})^\complement)$ is $1$-Lipschitz). Besides, we know that outside the ball $B_\varepsilon(0)$, the function $g$ is $(1/\varepsilon)$-Lipschitz. 
    
    Using the convexity function $z \mapsto \sum_{j \in \mathcal{A}_z} d(z, (A_j^{\varepsilon}))$ (as a sum of convex functions), we can show that for all $z \in \mathcal{A}_z$, we have that $f(z) \leqslant (k-1) \varepsilon$ and $f(z)$ is not $B_\varepsilon(0)$.  Finally, the function $h$ is $\frac{\sqrt{k}}{\varepsilon}$-Lipschitz.
    
    Thus, we have that:
    \begin{equation*}
        \|G(z) - G(z')\| \leqslant \frac{d \sqrt{k}}{\varepsilon} \|z - z'\|,
    \end{equation*}
    with $d = \underset{(i,j) \in [1,n]^2}{\max} \|X_i - X_j\|$.
    Consequently, noting that $\varepsilon = \frac{d \sqrt{m}}{L}$, we have that:
    \begin{equation*}
        \|G(z) - G(z')\| \leqslant L \|z - z'\|.
    \end{equation*}
    We consequently finally conclude on the Lipschitzness of $G^\star$ on $\mathds{R}^d$.
    
    The precision $\text{precision}$ of $G^\star$ is thus such that:
    \begin{equation*}
        \text{precision} = 1 - \gamma(\partial^\varepsilon \mathcal{A}).
    \end{equation*}
    However, since $\partial^\varepsilon \mathcal{A} \subset \bigcup_{i=1}^n A_i^\epsilon$, we have that
    %$\big( \cup_{j \neq i} A_j\big)^\varepsilon \textbackslash \big(\cup_{j \neq i} A_j \big)$ is disjoint, we have that:
    \begin{align*}
        \gamma(\partial^\varepsilon \mathcal{A}) &\leqslant \sum_{i=1}^n \gamma(A_i^\varepsilon).
    \end{align*}
    Using results from \citet[][Corollary 1]{schechtman2012approximate}, we have that
    \begin{equation*}
        \gamma(A_i^\varepsilon) \leqslant \frac{\varepsilon}{2n} \big(\sqrt{\pi \log(Lm)} + O(\frac{\log(L)}{L}) \big)  
    \end{equation*}
    Thus, we have
    \begin{equation*}
        \text{precision} \geqslant 1 - (\varepsilon/2) \big(\sqrt{\pi \log(Lm)} + O(\frac{\log(L)}{L}) \big) .
    \end{equation*}
    
    Now, let $n>d$. Consequently, for a fixed number of modes, we expect the precision to decrease when the dimension of the latent decreases. In particular, \citet{boland1995separating} have shown the number of hyperplanes $h$ required to separate $m$ points in a $d$ Euclidean space is such that:
    \begin{equation*}
        h \leqslant \lceil (m-2^{\lceil \log(d) \rceil}) / d)\rceil + \lceil \log(d) \rceil
    \end{equation*}
    Consequently, the optimal boundary has a measure lower than the union one the extension of these $h$ hyperplanes: 
    \begin{align*}
        \gamma_d \leqslant h \ \gamma_n(H^\varepsilon) \leqslant 
        \frac{\log(d) \varepsilon}{\sqrt{2\pi}} + O(\frac{m\varepsilon}{d}).
    \end{align*}
    Assuming that $\frac{m}{d} = o(\log(d))$, we have that the optimal generator has the following lower-bound:
    \begin{equation}\label{eq:prec_general_case}
        \alpha \geqslant 1 - \frac{\varepsilon \log(d)}{\sqrt{2 \pi}},
    \end{equation}
\end{proof}

\section{Evaluating GANs}
\subsection{Understanding the Density/Coverage}
\begin{definition}
    Let $X, Y$ be two random variables and $D_X, D_Y$ two finite sample datasets such that $D_X \sim X^n$ and $D_Y \sim Y^n$. For any $k \in \mathds{N}$ and $x \in D_X$, the density is defined as
\begin{equation*}
    \text{density} := \frac{1}{kM} \sum_{j=1}^M \ \sum_{i=1}^N \mathds{1}_{ \{Y_j \in \mathds{B}(X_i,k) \} }
\end{equation*}
where k is for the k-nearest neighbourhoods. Besides, 
\begin{equation*}
    \text{coverage} := \frac{1}{N} \sum_{i=1}^N \mathds{1}_{ 
    \{\exists j \in [1,M], Y_j \in \mathds{B}(X_i, k)\} }
\end{equation*}
\end{definition}
On the one hand, density focuses on whether the generated distribution can sample within high-density areas of the target distribution. On the other, coverage focuses on the support estimation part of the target distribution. 

These two proposed metrics are very useful for the evaluation of GANs. To better understand their use and objective, we propose the following asymptotic theorems:

\begin{theorem}
    Let $X, Y$ be two random variables and $D_X, D_Y$ two finite sample datasets such that $D_X \sim X^n$ and $D_Y \sim Y^n$. Let $(k,n)$ be such that $\frac{k}{\log(n)} \to 0$ and $\frac{k}{n} \to 0$. 
    \begin{enumerate}
        \item If $X$ is uniformly distributed, then $\text{density} \propto Y(S_X)$ (where $S_Y$ refers to the support of the random variable $Y$). 
        \item Then, $\text{coverage} \to X(S_Y)$.
    \end{enumerate}
\end{theorem}

Even these two metrics seem to empirically improve upon the Precision/Recall metric \citep{naeem2020reliable}, we believe one key element is still missing from this evaluation scheme: evaluating whether two neighborhoods with relatively same density of samples also contain the same number of generated/fake samples. Indeed, we argue that one of the main drawbacks of the Density/Coverage metric from \cite{naeem2020reliable}, is that it is not sensible to partial mode collapse. Indeed, we define in Figure \ref{fig:partial_mode_collapse}, two synthetic cases:
\begin{enumerate}
    \item In the first one, each mode of the target distribution is covered equally, and we observe $\text{density} = \text{coverage} =1$.
    \item In the second case, every mode is covered but the coverage is highly unequal. However, using the density/coverage metric we still have $\text{density}=\text{coverage}=1$.
\end{enumerate}
\begin{figure}[h]
    \centering
    \includegraphics[scale=0.1]{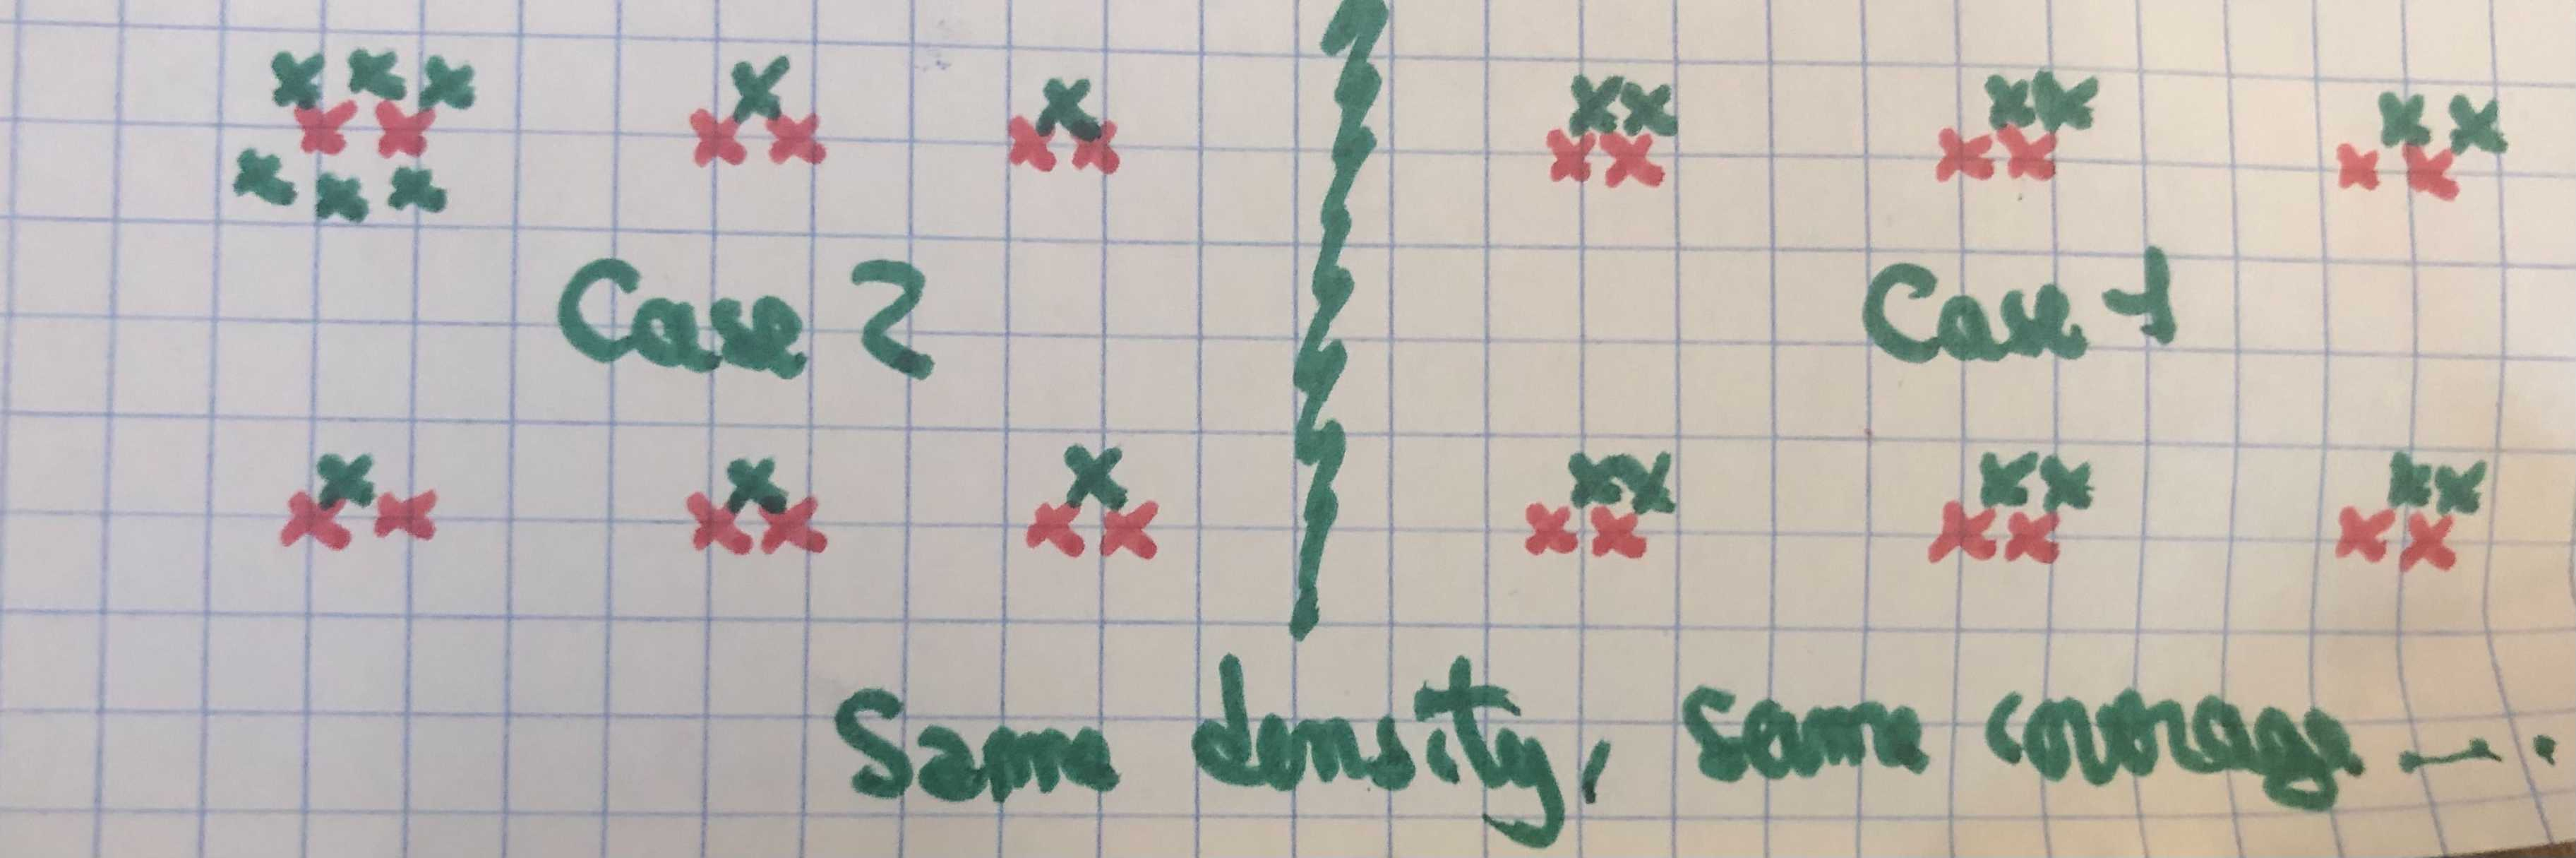}
    \caption{Example \label{fig:partial_mode_collapse}}
\end{figure} 

\subsection{The equilibrium metric}
To solve this, we propose to add the equilibrium measure. It relies on the idea that a similar number of fake points should belong to the different neighborhoods of $X_i, i \in [1, N]$. More precisely, we advocate that each region of the Voronoi diagram formed by $(X_1, \hdots, X_n)$ should contain the same number of fake points $Y_i, i \in [1, M]$. 

To properly measure equilibrium, we therefore need the use the following definition of Voronoi diagrams:
\begin{definition}
For a given euclidean space $\mathds{R}^D$ ($d \in \mathds{N}$), the Voronoi diagram $\mathscr{W} = \{ W(X_1), \hdots, W(X_n) \}$ of the dataset $X_1, \hdots, X_n \in (\mathds{R}^D)^n$ is defined by: 
\begin{equation*}
    \text{for all i} \in [1,n], \ W(X_i) = \{ x \in \mathds{R}^D: \|X_i-x\| = \underset{j \in [1,n]}{\min} \ \|X_j-x\| \}
\end{equation*}
\end{definition}
Finally, to quantify the dispersion, we use a divergence
\begin{definition}
    Let $X, Y$ be two random variables and $D_X, D_Y$ two finite sample datasets such that $D_X \sim X^n$ and $D_Y \sim Y^n$. For any $k \in \mathds{N}$ and $x \in D_X$, the density is defined as
\begin{equation*}
    \text{Equilibrium} := KL \Big(\mathds{U} || \frac{\text{card}(\{Y_j \in [1, M], Y_j \in W(X_i) \}_{i \in [1, N]})}{N} \Big)
\end{equation*}
where k is for the k-nearest neighbourhoods. 
\end{definition}

% \subsection{Proof of Theorem }
% We want to determine the number of hyperplanes required to separate $n$ distincts points in $\mathds{R}^d$. 
% It is well known that the maximal number of regions $n_{\text{max}}$ created by the separation of $h$ hyperplanes in $\mathds{R}^d$ (where $h \geqslant d$) is equal to:
% \begin{equation*}
%     n_{\text{max}}(h,d) = \sum_{i=0}^d \ {h \choose i}.
% \end{equation*}
% In this setting, we have $n_{\text{max}}(h,d) = 2^d$ when $h=d$. Consequently, if $n\leqslant 2^d$, it requires at least $d = \log_2(n)$ hyperplanes to separate those $n$ points. The optimal boundary has a measure lower than the union one of $n$ hyperplanes intersecting in $0$: 
% \begin{align*}
%     \gamma_d \leqslant d \gamma_n(H^\varepsilon) \leqslant \Big( \frac{d \varepsilon}{\sqrt{2 \pi}}\Big),
% \end{align*}
% meaning the optimal generator has a precision bigger than:
% \begin{align*}
%     \alpha \geqslant 1 - \frac{d \varepsilon}{\sqrt{2 \pi}}
% \end{align*}
% Now, if $n > 2^d$, it requires more than a number $h \geqslant d$ of hyperplanes to separate the $n$ distinct points. We have
% \begin{equation*}
%     n_{\text{max}}(h,d) = \sum_{i=0}^d \ {h \choose i} \geqslant \sum_{i=0}^d \Big(\frac{h}{i} \Big)^i \geqslant \Big(\frac{h}{d} \Big)^d
% \end{equation*}
% And thus, we have that it requires at most:
% \begin{equation*}
%     h \leqslant d n^{1/d}
% \end{equation*}
% hyperplanes to separate those $n$ points, i.e. meaning the optimal generator has a precision bigger than:
% \begin{align*}
%     \alpha \geqslant 1 - \frac{d n^{1/d} \varepsilon}{\sqrt{2 \pi}}
% \end{align*}


Now, let $m>d$. Consequently, for a fixed number of modes, we expect the precision to decrease when the dimension of the latent space decreases. In particular, \citet{boland1995separating} have shown the number of hyperplanes $h$ required to separate $m$ points in a $d$ Euclidean space is such that:
    \begin{equation*}
        h \leqslant \lceil (m-2^{\lceil \log(d) \rceil}) / d)\rceil + \lceil \log(d) \rceil
    \end{equation*}
    
    Consequently, the optimal boundary $\mathcal{A}^\star$ has a measure lower than the union of the extension of these $h$ hyperplanes: 
    \begin{align*}
        h \gamma (H^\varepsilon)  \leqslant (\frac{m}{d} + \log d + K) \times
        \frac{ \varepsilon}{\sqrt{2\pi}}, \text{where } 2 \leqslant K \leqslant 4.
    \end{align*}
    We thus have that the generator $G^\star_\varepsilon$ associated with $\mathcal{A}^\star$ is $L$-Lipschitz (Theorem \ref{th:optimal_precision_GANs}) has the following lower-bound:
    \begin{align*}
        \alpha_G 
        &\geqslant 1 - \gamma (\partial^\varepsilon(\mathcal{A}^\star)), \\ &\geqslant 1 - \frac{\varepsilon_{\text{max}} (\log(d) + \frac{m}{d})}{\sqrt{2 \pi}}+ O(\varepsilon_{\text{max}}).
    \end{align*}
    
    \subsection{Old part}
    Consequently, the optimal boundary $\mathcal{A}^\star$ has a measure lower than the union of the extension of these $h$ hyperplanes: 
    \begin{align*}
        h \gamma (H^\varepsilon) \leqslant 
        \frac{\log(d) \varepsilon}{\sqrt{2\pi}} + O(\frac{m\varepsilon}{d}).
    \end{align*}
    Assuming that $\frac{m}{d} = o(\log(d))$, we have that the generator $G^\star_\varepsilon$ associated with $\mathcal{A}^\star$ is $L$-Lipschitz (Theorem \ref{th:optimal_precision_GANs}) has the following lower-bound:
    \begin{align*}
        \alpha_G 
        &\geqslant 1 - \gamma (\partial^\varepsilon(\mathcal{A}^\star)), \\ &\geqslant 1 - \frac{\varepsilon_{\text{max}} \log(d)}{\sqrt{2 \pi}}+ O(\frac{m\varepsilon_{\text{max}}}{d}).
    \end{align*}
    
